# Supplementary material for: Investigating Non-linear and Stochastic Hard X-ray Variability of Active Galactic Nuclei using Recurrence Analysis
Source: arXiv:2211.13774 source file (2022-11-24)
Supplement: Supplementary file 2 [file MNRAS_SwiftBAT_RPs_Appendices.pdf]

## APPENDIX A: GENERATING A RECURRENCE PLOT: HER X-1

To demonstrate the construction of a RP and its important features (namely, diagonal lines), we will walk through a brief example. We consider the first 70 months of monitoring by *Swift*/BAT of the bright neutron star X-ray binary, Her X-1, which has a fairly consistent 35-day modulation associated with a precessing accretion disk (Staubert et al. 2009), displayed in Fig. A1. Here we binned the snapshot light curve every 5 days with a weighted mean of the total flux from all eight energy channels of the *Swift*/BAT telescope (details of the light curve construction are explained in Sec. 3 of the main body of the paper).

We use the Takens’ time delay method (Takens 1981) to embed the Her X-1 light curve into a higher dimensional phase. The time delay method maps the observations in the light curve,  $\vec{x}(t)$ , to the time-delay embedded vectors  $y(t) = (y_1(t), y_2(t), \dots, y_m(t))$ , where  $m$  is the dimension of the embedded vector and  $y_j(t) = x(t - \tau_j)$  for  $j = 1, 2, \dots, m$  are the embedded components. The time delay is defined as  $\tau = k\Delta t$ , where  $\Delta t$  is the cadence of the light curve. An appropriate choice for the time delay is one in which the time delay is longer than the linear or nonlinear correlation times in the time series (e.g., the autocorrelation time). We use the first minimum in the mutual information (Fraser & Swinney 1986) to choose an appropriate time delay, which is similar to the autocorrelation function but additionally probes nonlinear correlations. We use the false nearest neighbors method to determine the optimal dimension (Kennel et al. 1992). Further details of constructing phase space from AGN light curves using these methods can be found in Phillipson et al. (2020).

We embed the Her X-1 light curve into phase space using an embedding dimension of 15 and a time delay corresponding to 24 days and compute the recurrence matrix, Eq. 1 in the main body of the paper. The resulting recurrence plot for the Her X-1 light curve is displayed in Fig. A2 (top panel). We see that the 35-day period persistent in the Her X-1 source manifests as evenly spaced diagonal lines throughout the entire RP with subtle variations in structure.

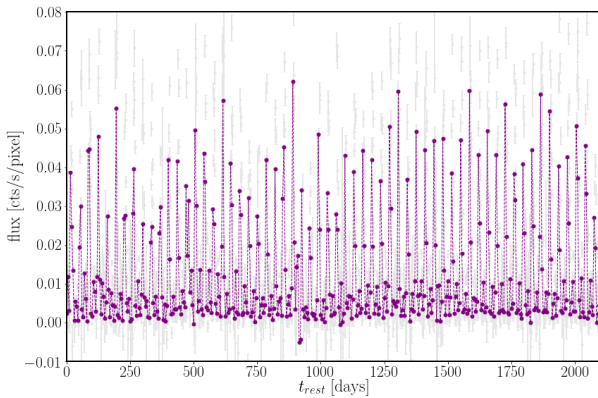

**Figure A1:** The 70-month 14-150 keV *Swift*/BAT light curve of Her X-1 binned to 5 days with a weighted average over the 8 energy bands. The snapshot light curve data points with associated errors are in grey, and the resulting binned light curve is in closed purple circles (dotted line).

For the 46 AGN detailed in Table 1 in the main body of

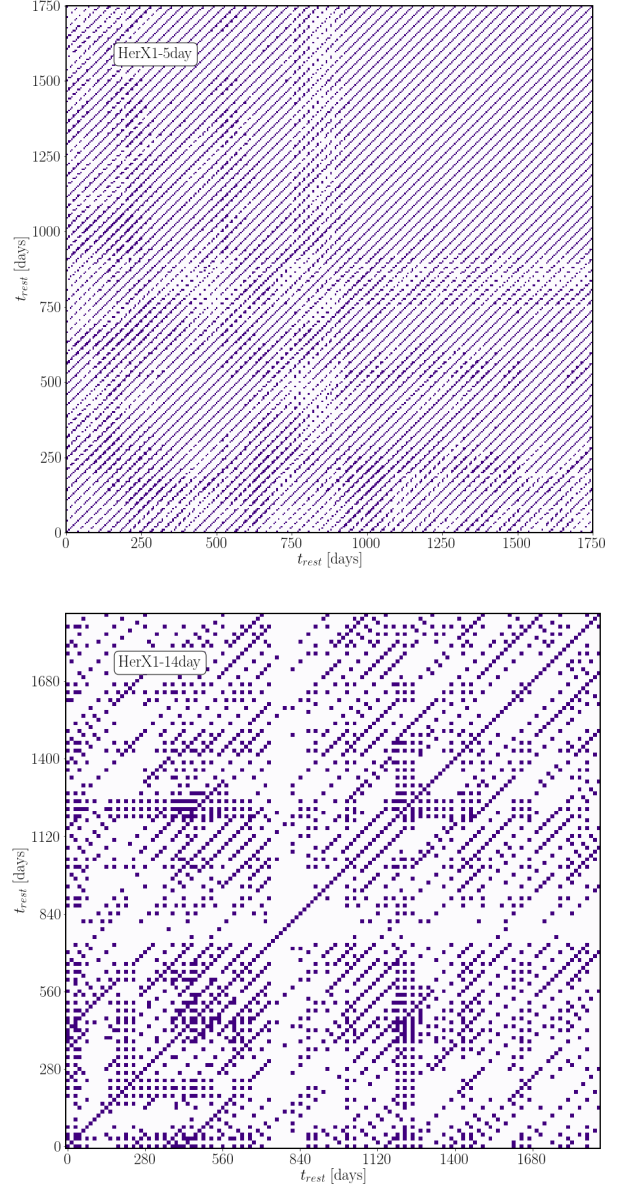

**Figure A2.** The recurrence plot of Her X-1 of the 5-day binned *Swift*/BAT light curve (top) and 14-day light curve (bottom) for a threshold corresponding to a recurrence rate of 15 percent. The average spacing between diagonal lines in the 5-day light curve RP is 35 days, corresponding to the intrinsic modulation time associated with the precessing disk in Her X-1. The average spacing in the diagonal lines for the 14-day light curve RP is 70 days, twice the fundamental period.

the paper, we determine appropriate embedding parameters using the same techniques. In the case of the time delay, if a pronounced minimum in the mutual information is not detected, we use the autocorrelation time instead. The time delays and embedding dimensions for all AGN are listed in Table A1.

Continuing with the example of Her X-1, we generate three types of surrogate time series: “Phase” surrogates are formed by Fourier transform, randomizing phase, and transforming back, thus preserving the PSD but with a Gaussian distribution of flux and no higher order moments. “Shuffled” surro-

**Table A1.** The embedding parameters of the *Swift*/BAT AGN. The embedding dimension is  $m$ , and the embedding time delay is defined as  $\tau = k\Delta t$ , where  $\Delta t$  is the cadence (or binning) of the light curve, 5 days for this sample.

| Object          | $k$ | $m$ |
|-----------------|-----|-----|
| 3C 111          | 3   | 4   |
| 3C 273          | 4   | 4   |
| 3C 382          | 3   | 4   |
| 3C 454.3        | 3   | 4   |
| 4C 50.55        | 3   | 4   |
| 4U 0557-38      | 3   | 4   |
| 4U 1344-60      | 3   | 4   |
| Cen A           | 11  | 5   |
| Circinus Galaxy | 2   | 4   |
| Cygnus A        | 3   | 4   |
| ESO 103-035     | 2   | 4   |
| ESO 297-018     | 3   | 4   |
| ESO 506-G027    | 3   | 4   |
| GRS 1734-292    | 5   | 5   |
| IC 4329A        | 3   | 5   |
| MCG+08-11-011   | 5   | 4   |
| MCG-05-23-016   | 3   | 5   |
| MR 2251-178     | 3   | 5   |
| Mrk 6           | 3   | 4   |
| Mrk 110         | 3   | 5   |
| Mrk 348         | 3   | 5   |
| Mrk 421         | 3   | 4   |
| Mrk 926         | 5   | 5   |
| NGC 1275        | 4   | 5   |
| NGC 1365        | 2   | 4   |
| NGC 2110        | 17  | 5   |
| NGC 2992        | 5   | 5   |
| NGC 3081        | 2   | 4   |
| NGC 3281        | 3   | 4   |
| NGC 3516        | 2   | 5   |
| NGC 3783        | 2   | 4   |
| NGC 4151        | 6   | 5   |
| NGC 4388        | 8   | 4   |
| NGC 4507        | 3   | 4   |
| NGC 4593        | 8   | 6   |
| NGC 4945        | 3   | 4   |
| NGC 5252        | 4   | 4   |
| NGC 5506        | 3   | 5   |
| NGC 5548        | 3   | 5   |
| NGC 5728        | 2   | 5   |
| NGC 6814        | 3   | 5   |
| NGC 7172        | 3   | 5   |
| NGC 7582        | 3   | 4   |
| PKS 0018-19     | 3   | 4   |
| QSO B0241+622   | 3   | 5   |
| XSS J05054-2348 | 2   | 5   |

gates are formed by shuffling the time ordering of the flux values from the light curve, thus preserving the flux distribution, but removing all correlations. And the “IAAFT” surrogates are generated from the iteratively amplitude adjusted Fourier transform algorithm (Schreiber & Schmitz 1996), which preserves both the flux distribution and the PSD. The foundation of the surrogate data method is that the method of generating surrogates always destroys dynamical information while retaining certain statistical properties; thus, distinct behavior between data and surrogates indicates it is not generated from the null hypothesis that corresponds to the surrogate generation method. For example, the shuffled surrogates correspond to a null hypothesis that the time series is produced

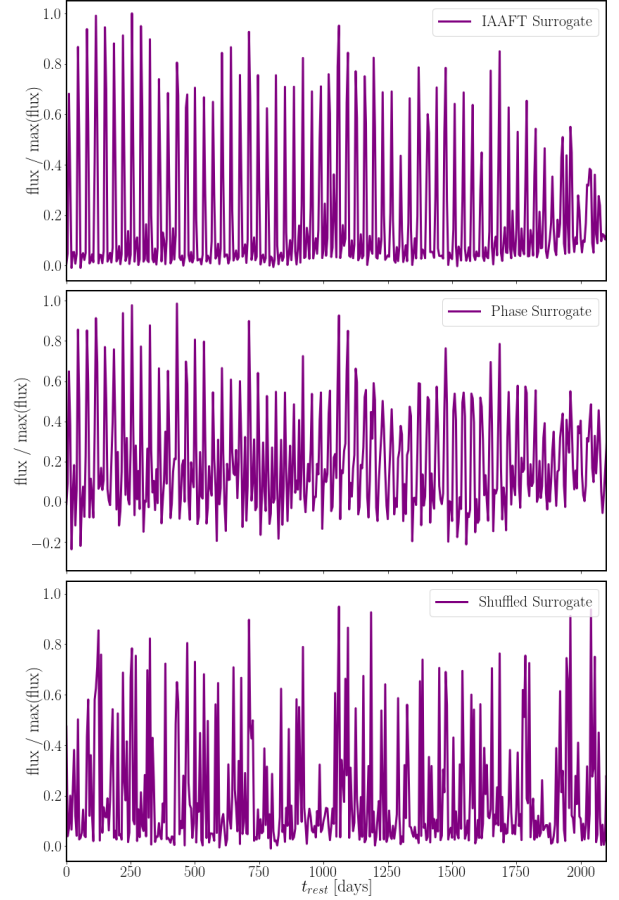

**Figure A3.** Three example surrogate time series of the Her X-1 light curve: (top) an IAAFT surrogate preserving both the PSD and the flux distribution, (middle) a phase surrogate preserving the PSD but not the flux distribution (a randomization of the phases in Fourier space), and (bottom) a shuffled surrogate preserving only the flux distribution while destroying the time-ordering information.

from an independent and identically distributed noise process. We use the nonlinear time series analysis code, *TISEAN* (Hegger et al. 1999, Schreiber & Schmitz 2000) for generating 100 surrogates of each type. Examples of each type of surrogate for the Her X-1 light curve are plotted in Fig. A3.

To test the null hypothesis corresponding to each type of surrogate and determine whether higher order modes are present in the Her X-1 light curve, we use measures from the RP as the test statistic. For each of the three types of surrogate data and the Her X-1 light curve, we generate the RP using the same time delay embedding parameters and calculate one quantity from the RP that is an indicator of nonlinearity: the length of the longest diagonal line,  $L_{max}$ . For systems that contain higher determinism and nonlinearity,  $L_{max}$  should be systematically higher, as it is related to the largest Lyapunov exponent describing an attractor in phase space (Eckmann et al. 1987). Fig. B1 displays the  $L_{max}$  measure as a function of threshold ( $\epsilon$  in Eq. 1 in the main body of the paper) for both the Her X-1 light curve and 3 types of surrogates (top panel), where we see the longest diagonal line is consistently larger than the ensemble of surrogates of all three types. Using the rank-order significance test described

in Sec. 4 in the main body of the paper, the  $L_{max}$  measure for the data is ranked in the top 5 per cent compared to all surrogates over a wide range of threshold. These results support the model that the underlying mechanism driving the 35-day modulation is due to a nonlinear process, such as a precessing warped accretion disk.

## APPENDIX B: BINNING AND SIGNAL-TO-NOISE REQUIREMENTS

We consider two very bright X-ray binaries for which physical timescales are well defined and whose light curves evident behavior typical for study with recurrence analysis (e.g., quasi-periodicity). We will determine the level of noise and width of time bins for which the deterministic behavior is no longer detectable with recurrence analysis.

The two objects chosen are Her X-1, introduced in Sec. A, and SMC X-1, which has an orbital variation at 3.98 days (Schreier et al. 1972) and a super-orbital modulation between 45 and 60 days (Wojdowski et al. 1998). We re-bin the raw light curves of each object into time bins with widths of 1 day, 3 days, 5 days, 7 days, 10 days, and 14 days. We find that 5-day or shorter binning is required in order to recover the 35-day periodicity of Her X-1 and orbital modes of SMC X-1 in the RPs of both objects. An example RP of Her X-1 in Fig. A2 for a time binning of 5 days and of 14 days exemplifies the disappearance of the 35-day periodicity in the longer binning time.

The second important criterion for recurrence analysis is a signal-to-noise threshold in the time series. Previous work explored the role of noise in detecting deterministic recurrences by systematically adding synthetic noise to time series of simulated chaotic and periodic orbits in disks around black holes (Suková et al. 2016). Recurrence analysis failed to distinguish the periodic orbits above a 25 per cent noise level (where added noise is as a fraction of the signal variance), and fails to detect chaotic orbits above 100 per cent added noise. We follow a similar approach in determining an appropriate signal-to-noise requirement for analysis of the *Swift*/BAT light curves. We use the 5-day binned light curves of Her X-1 and SMC X-1, which are expected to have light curves similar to the “regular” orbits modeled by the Suková et al. team. We added noise in increments from 10 per cent to 100 per cent of the original light curve variance and use the surrogate data method to determine the significance of structure in the RP compared to three sets of surrogate data.

The test statistic used to distinguish data from surrogates is the longest diagonal line length ( $L_{max}$ ) and the determinism ( $DET$ ). If the values of these metrics are distinct from the sets of surrogates for a wide range of thresholds ( $\epsilon$  in Eq. 1 in the main body of the paper), then we can say that the light curves likely contain higher-order, deterministic modes connected to the physical timescales in these objects. In Fig. B1 we show the longest diagonal line length as a function of threshold for Her X-1 against 100 surrogates of each surrogate type (shuffled, phase, and IAAFT). Above 50 per cent noise, the algorithm used to determine a proper embedding dimension fails (the false nearest neighbors method; Kennel et al. 1992). Above a 25 percent noise level, the  $L_{max}$  measure in particular begins to fail to distinguish the data from the surrogates with high significance. We therefore conclude

that a minimum signal-to-noise ratio of 5 is appropriate for our applications of recurrence analysis on *Swift*/BAT 5-day binned light curves. 657 of the *Swift*/BAT AGN are above this threshold in the 157-month catalog, and all 46 AGN selected for this study are well above this threshold.

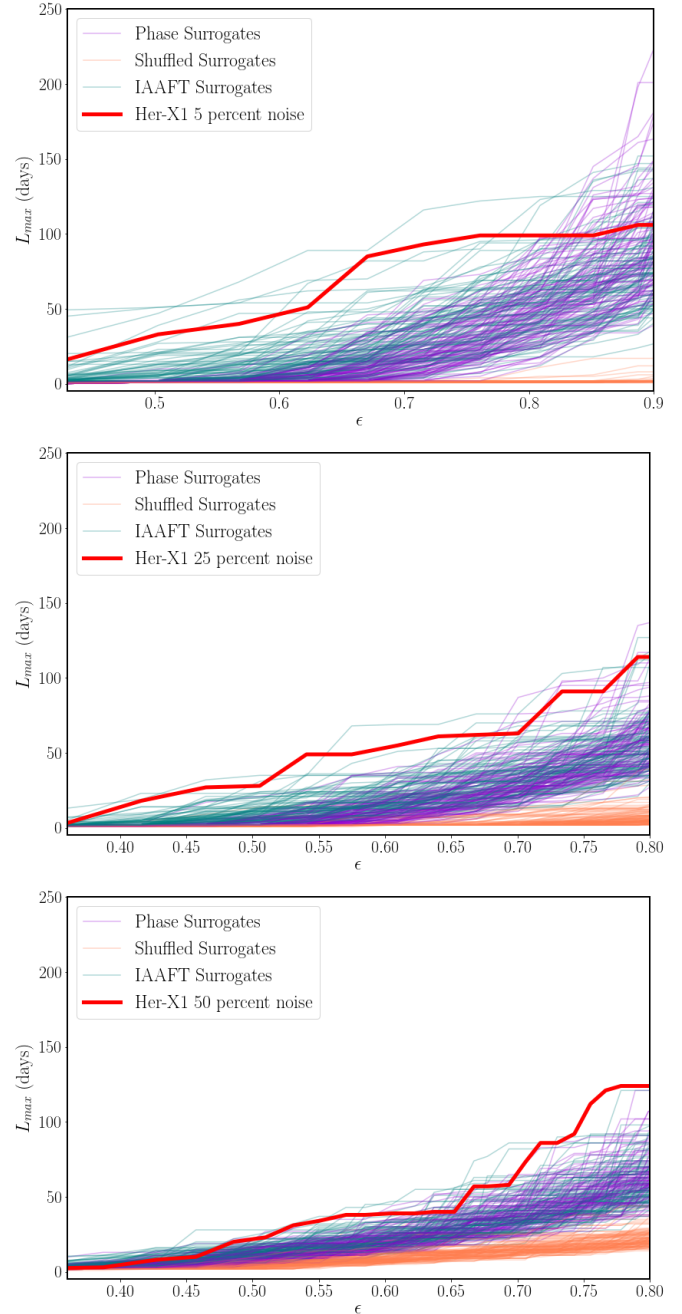

**Figure B1:** The longest diagonal line length,  $L_{max}$ , computed from the recurrence plot of Her X-1 for a range of thresholds between approximately 1 percent recurrence rate up to 70 percent recurrence rate for different amounts of added noise (as a fraction of total variance in the light curve): (top) 5 percent, (middle) 25 percent, and (bottom) 50 percent added noise. By about 50 percent added noise, the  $L_{max}$  measure becomes indistinguishable from the ensemble of surrogates at the lowest thresholds. This effect worsens with increasing added noise.

## APPENDIX C: SYSTEMATICS

We consider the 106 Blank Sky light curves provided by the *Swift*/BAT transient monitor in order to study spurious features that may arise in the recurrence plot due to the light curve preparation methods or recurrence plot construction. We compute the time-delayed mutual information (Fraser & Swinney 1986) of all of the blank sky light curves using the TISEAN package ‘mutual’ functionality. The mutual information is defined as:

$$S = - \sum_{ij} p_{ij}(\tau) \ln \frac{p_{ij}(\tau)}{p_i p_j}, \quad (\text{C1})$$

where, for some partition on the real numbers of evenly spaced intervals,  $p_i$  is the probability to find a time series value in the  $i$ -th interval, and  $p_{ij}(\tau)$  is the joint probability that an observation falls into the  $i$ -th interval and the observation time  $\tau$  later falls into the  $j$ -th interval (Hegger et al. 1999).

Among the blank sky light curves we observe a systematic yearly timescale which is evidently associated with the occurrence of gaps in the observations. In Fig. C1 we provide three examples of typical behavior seen in the mutual observation of the blank sky light curves. In some light curves, the systematic does not appear (roughly two thirds of the blank sky light curves). Others exhibit a modest systematic (top panel of Fig. C1), strongly evident systematic (middle panel), or an additional sub-harmonic at half the period (bottom panel). We also note that these timescales do not necessarily appear in the autocorrelation function, plotted with each example mutual information function.

We observe a similar systematic in a handful of the AGN in our sample, as seen in Fig. C2. Those that show a weak systematic in the mutual information include: 3C 111, 3C 273, MCG +08-11-011, Mrk 926, and NGC 5506; a moderate to strong systematic appears in GRS 1734-292, MR 2251-178, NGC 4593, and NGC 5728. Three examples of the mutual information and autocorrelation function are displayed in Fig. C3, where we show sources that contain a weak (3C 111), moderate (MR 2251-178), and strong (NGC 4593) systematic.

We explore the impact of these systematic gaps in the AGN light curves on the recurrence plot by constructing the Close Returns histogram (Phillipson et al. 2020). The recurrence rate along a specific diagonal of the recurrence plot is defined as:

$$RR_\kappa = \frac{1}{N - \kappa} \sum_{i=1}^{N-\kappa} \mathbf{R}_{i,i+\kappa}, \quad (\text{C2})$$

where  $\mathbf{R}$  is the recurrence matrix,  $N$  is the size of the recurrence matrix, and  $\kappa$  is the offset from the main diagonal of the recurrence plot. The close returns histogram,  $H(\kappa)$ , is the histogram of  $RR_\kappa$  for all offsets,  $\kappa$ , from the main diagonal. In other words, it is the summation along the diagonals of the recurrence matrix and can be viewed as a pseudo-autocorrelation function. Three examples of the close returns histogram are displayed in Fig. C3 that correspond to the same sources shown in Fig. C2. We note that the systematic that appears in the mutual information is greatly reduced in the close returns histogram. This is likely because the embedding process into phase space operates as a filter on the light curve, enhancing dynamics and dampening noise.

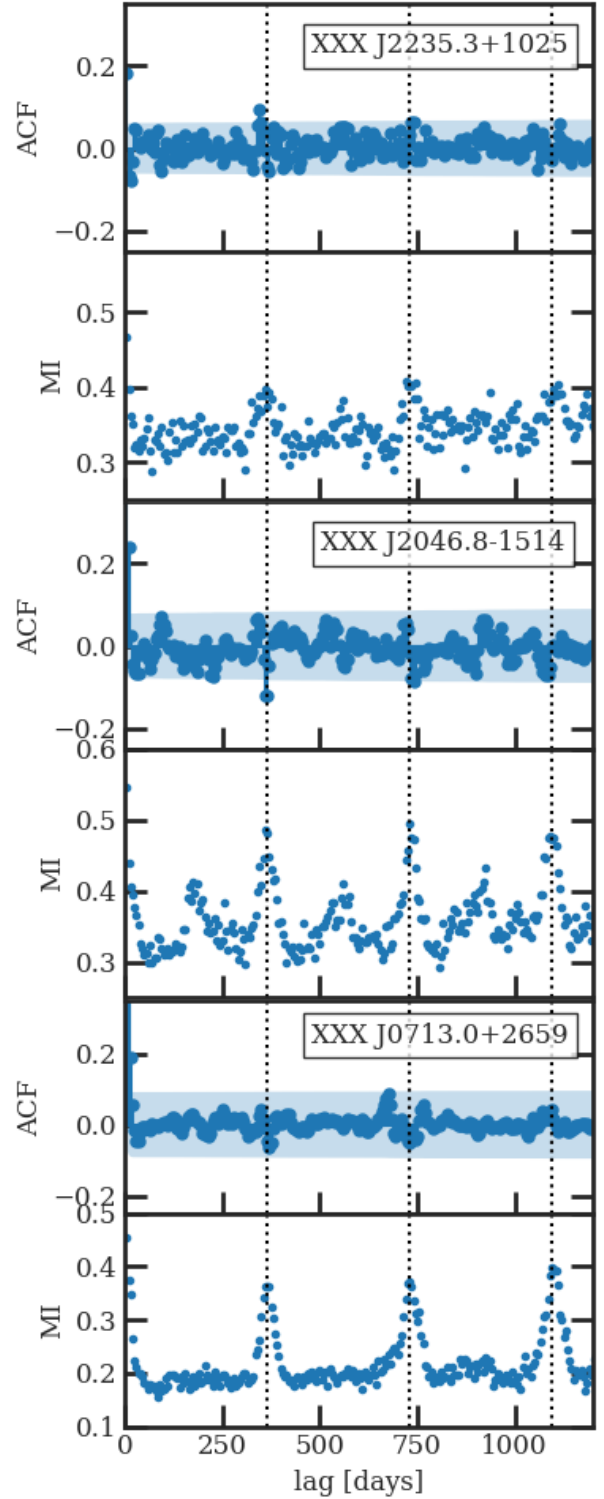

**Figure C1.** Three example autocorrelation functions, ACF, (top) and mutual information, MI, (bottom) where the systematic is modestly evident (J2235.3+1025), evident alongside a sub-harmonic (J2046.8-1514), and strongly evident (J0713.0+2659) in the MI and not necessarily in the ACF. The vertical dotted line in each figure is every 365 days.



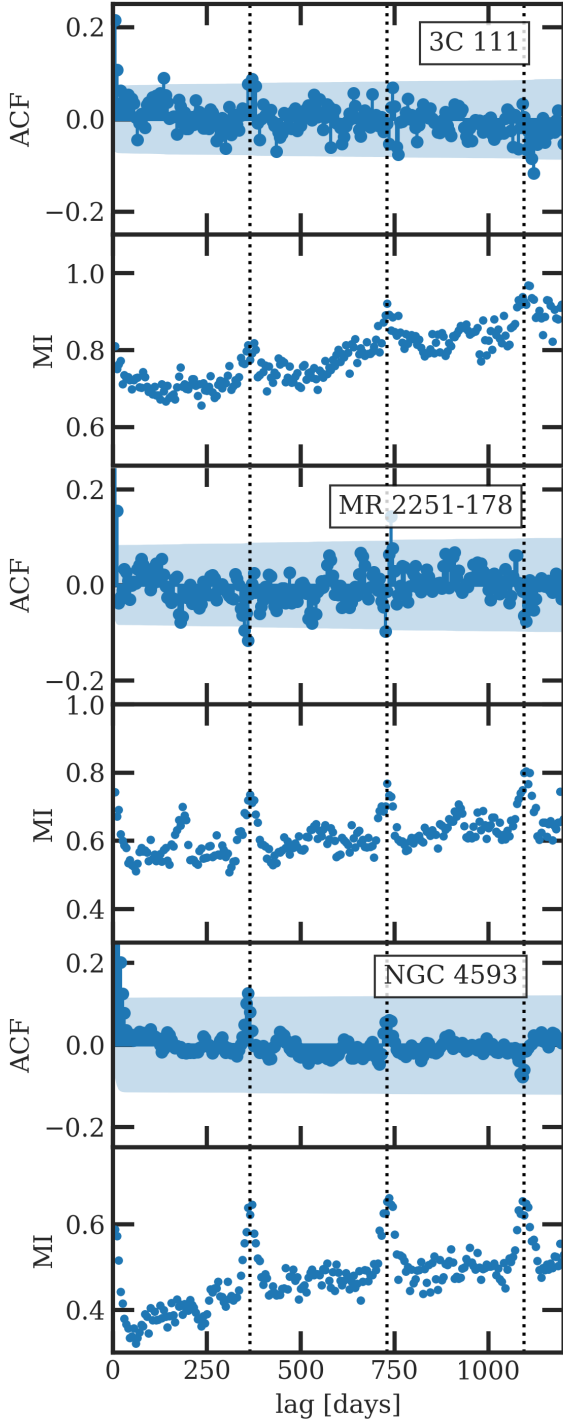

**Figure C2.** Three example autocorrelation functions, ACF, (top) and mutual information, MI, (bottom) where the systematic is modestly evident (3C 111), evident alongside a sub-harmonic (MR 2251-178), and strongly evident (NGC 4593) in the MI and not necessarily in the ACF. The vertical dotted line in each figure is every 365 days.

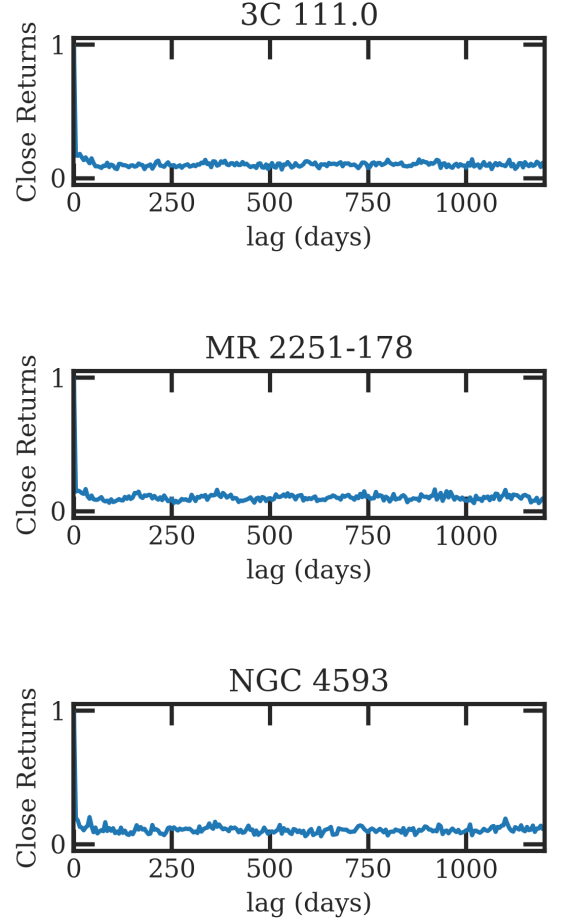

**Figure C3.** The close returns,  $H(\kappa)$  (Eq. C2), of sources with a detected systematic from Fig. C2. Similar to an autocorrelation function normalized to run between zero and unity, peaks in the close returns correspond to strong correlations. The systematic is most evident in MR 2251-178, but all cases is reduced compared to the mutual information or autocorrelation function.

Finally, we note that there are two sources, Cen A and NGC 2110, for which a timescale in the close returns histogram appears that may not be associated with the 365 day systematic. We show the close returns histograms in Fig. C4 where we observe a  $\sim 1000$  day signal. It may be possible to use the close returns analysis to determine non-yearly timescales that may appear in the full sample of *Swift*/BAT AGN. For the purposes of this study, we find that the embedding process and recurrence plot generation damps the signals evident in the mutual information. Furthermore, the use of the surrogate data method is critical for determining significance of any feature present in the recurrence plots because the surrogate data themselves are imprinted with the same systematics as the light curves. That is, the preservation of the power spectrum in the phase and IAAFT surrogates in particular ensures any detection of prominent recurrence features, such as determinism or nonlinearity, is robust against noise or systematic influence.

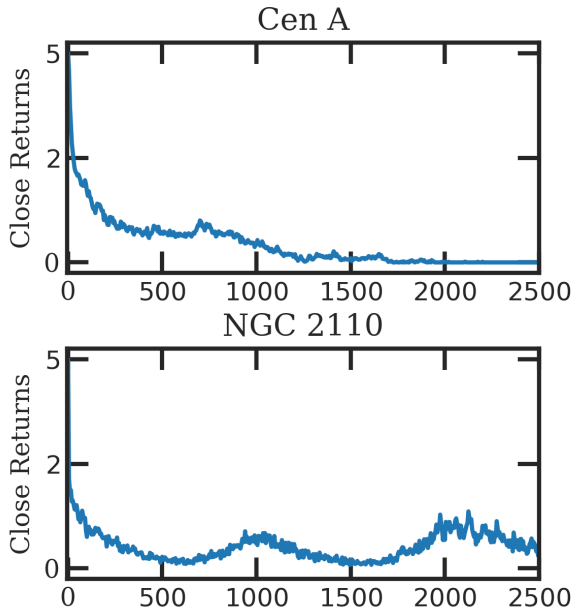

**Figure C4:** Close Returns of Cen A (top) and NGC 2110 (bottom) which both exhibit timescales distinct from systematic at 365 days. Cen A is considered non-stationary from its recurrence plot, while NGC 2110 passed all stationarity tests (Sec. 4 in the main body of the paper).

## REFERENCES

- Eckmann J.-P., Oliffson Kamphorst S., Ruelle D., 1987, *EPL*, 4, 973
- Fraser A. M., Swinney H. L., 1986, *Phys. Rev. A*, 33, 1134
- Hegger R., Kantz H., Schreiber T., 1999, *Chaos*, 9
- Kennel M. B., Brown R., Abarbanel H. D. I., 1992, *Phys. Rev. A*, 45
- Phillipson R. A., Boyd P. T., Smale A. P., Vogeley M. S., 2020, *MNRAS*, 497, 3418
- Schreiber T., Schmitz A., 1996, *PRL*, 77, 635
- Schreiber T., Schmitz A., 2000, *Physica D*, 142
- Schreiber E., Giacconi R., Gursky H., Kellogg E., Tananbaum H., 1972, *ApJL*, 178, L71
- Staubert R., Klochkov D., Postnov K., Shakura N., Wilms J., Rothschild R. E., 2009, *A&A*, 494, 1025
- Suková P., Grzedzielski M., Janiuk A., 2016, *A&A*, 586
- Takens F., 1981, *Lect. Notes Math*, Berlin Springer Verlag, 898, 366
- Wojdowski P., Clark G. W., Levine A. M., Woo J. W., Zhang S. N., 1998, *ApJ*, 502, 253
